# Supplementary material for: Free-T2M: Robust Text-to-Motion Generation for Humanoid Robots via Frequency-Domain
Source: arXiv:2501.18232 source file (2025-11-10)
Supplement: Supplementary file 1 [file X_suppl.tex]

\clearpage
% \appendix
\onecolumn

\subsection{Overview of Appendix}
The Appendix is organized into the following sections:

\begin{itemize}

    \item Section~\ref{sec:Theorem}: Derivation and Proof.

    \item Section~\ref{sec:evalmetrics}: Evaluation Metrics.

    \item Section~\ref{efficiency}: Efficiency Analysis.
    \item Section~\ref{More visualization}: More Visualization Results.
    \item Section~\ref{data analysis}: Motion Data Analysis.
    \item Section~\ref{more experiments}: More Experiments, including loss coefficient ablation, different training methods, R-Precision under different sample sizes, mask strategy ablation.
    \item Section~\ref{app:human_eval}: Details of Human Evaluation.
\end{itemize}

\section{Derivation and Proof}
\label{sec:Theorem}

\subsection{Power Spectral Density in Diffusion Process}

\begin{theorem}[Power Spectral Density in Diffusion Process]
\label{theorem:psd_derivation}
In the forward diffusion process, the spectral density of the power $ S_{\mathbf{m}_t}(\omega) $ of the motion signal $\mathbf{m}_t$ at time $t$ can be expressed as:
\begin{equation}
    S_{\mathbf{m}_t}(\omega) = |\hat{\mathbf{m}}_0(\omega)|^2 + \int_0^t g^2(s)\mathrm{d}s,
\end{equation}

where $|\hat{\mathbf{m}}_0(\omega)|^2$ is the initial power spectral density of the motion signal, and $ \int_0^t g^2(s)\mathrm{d}s $ represents the accumulated noise energy in the frequency domain.
\end{theorem}

In the Time Domain, the forward diffusion process of Diffusion \cite{Sposini_2020} is defined as :
\begin{equation}
    \mathrm{d}\mathbf{m}_t = \mathbf{f}(\mathbf{m}_t, t)\mathrm{d}t + g(t)\mathrm{d}\mathbf{w}_t
\end{equation}

where $ \mathbf{f}(\mathbf{m}_t, t) $ is the drift coefficient, $ g(t) $ is the diffusion coefficient, and $ \mathbf{w}_t $ is the Wiener process. Assuming $ \mathbf{f}(\mathbf{m}_t, t) = 0 $, the integral form becomes:
\begin{equation}
    \mathbf{m}_t = \mathbf{m}_0 + \int_0^t g(s)\mathrm{d}\mathbf{w}_s
\end{equation}

Applying the discrete Fourier transform (DFT) to $\mathbf{m}_t$, we obtain:
\begin{equation}
    \hat{\mathbf{m}}_t(\omega) = \hat{\mathbf{m}}_0(\omega) + \hat{\boldsymbol{\epsilon}}_t(\omega)
\end{equation}

Where, $\hat{\mathbf{m}}_t(\omega)$ denotes the frequency-domain representation of $\mathbf{m}_t$, $\hat{\mathbf{m}}_0(\omega)$ represents the initial frequency-domain representation of the clean motion signal $\mathbf{m}_0$, and $\hat{\boldsymbol{\epsilon}}_t(\omega)$ corresponds to the frequency-domain representation of the noise term $\boldsymbol{\epsilon}_t$.

The noise term $\boldsymbol{\epsilon}_t$ in the time domain is:
\begin{equation}
    \boldsymbol{\epsilon}_t(x) = \int_0^t g(s)\mathrm{d}\mathbf{w}_s
\end{equation}

Using the autocorrelation property of the Wiener process, the expected value of the noise energy is:
\begin{equation}
    \mathbb{E}[\boldsymbol{\epsilon}_t(x)\boldsymbol{\epsilon}_t(y)] = 
\begin{cases}
\int_0^t g^2(s)\mathrm{d}s, & x = y, \\
0, & x \neq y
\end{cases}
\end{equation}

The Fourier transform of $\boldsymbol{\epsilon}_t(x)$ yields:
\begin{equation}
    \mathbb{E}[|\hat{\boldsymbol{\epsilon}}_t(\omega)|^2] = \int_0^t g^2(s)\mathrm{d}s
\end{equation}

So, the power spectral density $ S_{\mathbf{m}_t}(\omega) $ of the motion signal $\mathbf{m}_t$ is defined as:
\begin{equation}
    S_{\mathbf{m}_t}(\omega) = \mathbb{E}[|\hat{\mathbf{m}}_t(\omega)|^2]
\end{equation}

Substituting $\hat{\mathbf{m}}_t(\omega) = \hat{\mathbf{m}}_0(\omega) + \hat{\boldsymbol{\epsilon}}_t(\omega)$, we expand:
\begin{equation}
    \mathbb{E}[|\hat{\mathbf{m}}_t(\omega)|^2] = \mathbb{E}\left[|\hat{\mathbf{m}}_0(\omega)|^2 + 2\operatorname{Re}(\hat{\mathbf{m}}_0(\omega)\hat{\boldsymbol{\epsilon}}_t^*(\omega)) + |\hat{\boldsymbol{\epsilon}}_t(\omega)|^2\right]
\end{equation}

Since $\mathbb{E}[\hat{\boldsymbol{\epsilon}}_t(\omega)] = 0$ and $\mathbb{E}[\hat{\mathbf{m}}_0(\omega)\hat{\boldsymbol{\epsilon}}_t^*(\omega)] = 0$, the cross-term vanishes, leaving:
\begin{equation}
    S_{\mathbf{m}_t}(\omega) = |\hat{\mathbf{m}}_0(\omega)|^2 + \mathbb{E}[|\hat{\boldsymbol{\epsilon}}_t(\omega)|^2]
\end{equation}

Substituting $\mathbb{E}[|\hat{\boldsymbol{\epsilon}}_t(\omega)|^2] = \int_0^t g^2(s)\mathrm{d}s$, we arrive at:
\begin{equation}
    S_{\mathbf{m}_t}(\omega) = |\hat{\mathbf{m}}_0(\omega)|^2 + \int_0^t g^2(s)\mathrm{d}s
\end{equation}

This derivation demonstrates that the power spectral density of the motion signal at time $t$ comprises two components: the original signal power $|\hat{\mathbf{m}}_0(\omega)|^2$ and the noise power accumulated over time $\int_0^t g^2(s)\,\mathrm{d}s$.

\subsection{Spectral Analysis in Diffusion-Based Motion Generation}

\label{frequency_dynamics}
In the forward diffusion process for motion generation, high-frequency components are corrupted earlier than low-frequency components, while in the reverse denoising process, low-frequency components are reconstructed first, providing the semantic foundation for high-frequency recovery \cite{yang2022diffusionprobabilisticmodelslim}. Formally:

Given an initial motion signal $\mathbf{m}_0$, the power spectral density of the corrupted signal $\mathbf{m}_t$ at time $t$ (\ref{theorem:psd_derivation}) is expressed as 
\begin{equation}
    S_{\mathbf{m}_t}(\omega) = |\hat{\mathbf{m}}_0(\omega)|^2 + \int_0^t g^2(s)\,\mathrm{d}s,
\end{equation}
where $|\hat{\mathbf{m}}_0(\omega)|^2 \propto |\omega|^{-\alpha}$ with $\alpha > 0$, characterizing the low-pass nature of the motion data. The signal-to-noise ratio (SNR) at frequency $\omega$ is given by 
\begin{equation}
    \text{SNR}(\omega) = \frac{|\hat{\mathbf{m}}_0(\omega)|^2}{\int_0^t g^2(s)\,\mathrm{d}s},
\end{equation}
which reveals that the SNR decreases more rapidly at higher frequencies ($\omega_H$) compared to lower frequencies ($\omega_L$), highlighting the stronger impact of noise on high-frequency components of the motion signal.

\textbf{Forward Diffusion Process:}
The forward diffusion process corrupts the initial signal $\mathbf{m}_0$ by adding Gaussian noise over time. The stochastic differential equation (SDE) is:
\begin{equation}
\label{eq:diffusion_sde}
\mathrm{d}\mathbf{m}_t = \mathbf{f}(\mathbf{m}_t, t)\mathrm{d}t + g(t)\mathrm{d}\mathbf{w}_t,
\end{equation}
where $\mathbf{f}(\mathbf{m}_t, t)$ is the drift coefficient, $g(t)$ is the diffusion coefficient, and $\mathbf{w}_t$ is the Wiener process. Assuming $\mathbf{f}(\mathbf{m}_t, t) = 0$, the integral form is:
\begin{equation}
    \mathbf{m}_t = \mathbf{m}_0 + \int_0^t g(s)\mathrm{d}\mathbf{w}_s
\end{equation}

Applying the discrete Fourier transform (DFT), the frequency-domain representation is:
\begin{equation}
    \hat{\mathbf{m}}_t(\omega) = \hat{\mathbf{m}}_0(\omega) + \hat{\boldsymbol{\epsilon}}_t(\omega)
\end{equation}

where $\hat{\boldsymbol{\epsilon}}_t(\omega)$ is the noise component in the frequency domain.

The energy of $\hat{\boldsymbol{\epsilon}}_t(\omega)$ is:
\begin{equation}
    \mathbb{E}[|\hat{\boldsymbol{\epsilon}}_t(\omega)|^2] = \int_0^t g^2(s)\mathrm{d}s
\end{equation}

and the power spectral density of $\mathbf{m}_t$ is:
\begin{equation}
    S_{\mathbf{m}_t}(\omega) = |\hat{\mathbf{m}}_0(\omega)|^2 + \mathbb{E}[|\hat{\boldsymbol{\epsilon}}_t(\omega)|^2]
\end{equation}

Since $|\hat{\mathbf{m}}_0(\omega)|^2 \propto |\omega|^{-\alpha}$ for $\alpha > 0$, high-frequency components have significantly lower energy compared to low-frequency components. As $\int_0^t g^2(s)\mathrm{d}s$ increases over time, high-frequency components ($\omega_H$) are dominated by noise earlier than low-frequency components ($\omega_L$).

\textbf{Reverse Denoising Process:}
In the reverse process, the model reconstructs $\mathbf{m}_t$ by iteratively reducing noise. The denoising step, exemplified by DDPM \cite{DDPM}, is :
\begin{equation}
    \mathbf{m}_{t-1} = \sqrt{\alpha_{t-1}} \left( \frac{\mathbf{m}_t - \sqrt{1 - \alpha_t} \boldsymbol{\epsilon}_\theta(\mathbf{m}_t, t)}{\sqrt{\alpha_t}} \right) + \sqrt{1 - \alpha_{t-1}} \mathbf{z}
\end{equation}

where $\boldsymbol{\epsilon}_\theta(\mathbf{m}_t, t)$ is the predicted noise and $\mathbf{z}$ is Gaussian noise.

At high noise levels (early timesteps), the model primarily reconstructs low-frequency components ($\omega_L$) due to their higher SNR:
\begin{equation}
    \text{SNR}(\omega_L) > \text{SNR}(\omega_H)
\end{equation}

As noise reduces (later timesteps), the model can progressively recover high-frequency components ($\omega_H$), which are dependent on the reconstructed low-frequency foundation.

The hierarchical nature of signal recovery, where low frequencies provide the semantic structure and high frequencies refine details, is an inherent property of the diffusion model.

\subsubsection{Low-Frequency Preservation and High-Frequency Recovery in Motion Generation}

In motion generation, low-frequency components encode the semantic structure (e.g., walking or jumping) and must be preserved during early diffusion stages. High-frequency components, encoding fine details, are restored in later stages. Given an SNR threshold $\gamma$, the time $t_\gamma(\omega)$ at which SNR reaches $\gamma$ is defined as:
\begin{equation}
\label{eq:motion_snr_threshold}
\text{SNR}(\omega) = \frac{|\hat{\mathbf{m}}_0(\omega)|^2}{\int_0^{t_\gamma(\omega)} g^2(s)\mathrm{d}s} = \gamma.
\end{equation}

By solving for $t_\gamma(\omega)$, we can determine the recovery time for specific frequencies. So low-frequency components recover earlier, aligning with the semantic planning phase, while high-frequency components recover later, contributing to fine-grained details.

\subsection{Dependency of High-Frequency Components on Low-Frequency Structures in Motion Generation}

\label{hf_dependency}
In the reverse denoising process of diffusion models for motion generation, the accurate restoration of high-frequency motion details depends explicitly on the prior reconstruction of low-frequency semantic structures \cite{boostingdiffusionmodelsmoving}. Formally, let $\hat{\mathbf{m}}_t(\omega)$ denote the motion signal at timestep $t$ in the frequency domain, where $\omega$ represents the frequency. The recovery of high-frequency components $\hat{\mathbf{m}}_t(\omega_H)$ at frequency $\omega_H$ requires conditioned restoration based on the low-frequency components $\hat{\mathbf{m}}_t(\omega_L)$ at frequency $\omega_L$, such that:
\begin{equation}
    p(\hat{\mathbf{m}}_{t-1}(\omega_H) \mid \hat{\mathbf{m}}_t(\omega_H), \hat{\mathbf{m}}_t(\omega_L)) \approx p(\hat{\mathbf{m}}_{t-1}(\omega_H) \mid \hat{\mathbf{m}}_{t-1}(\omega_L))
\end{equation}

To analyze the dependency, consider the denoising process in diffusion models where motion data evolves from pure noise $\hat{\mathbf{m}}_T(\omega)$ back to the original signal $\hat{\mathbf{m}}_0(\omega)$ through iterative refinement:
\begin{equation}
    \hat{\mathbf{m}}_{t-1}(\omega) = \sqrt{\alpha_{t-1}} \left( \frac{\hat{\mathbf{m}}_t(\omega) - \sqrt{1 - \alpha_t} \boldsymbol{\epsilon}_\theta(\hat{\mathbf{m}}_t, t)}{\sqrt{\alpha_t}} \right) + \sqrt{1 - \alpha_{t-1}} \mathbf{z}
\end{equation}

where $\boldsymbol{\epsilon}_\theta$ is the neural network's predicted noise, $\alpha_t$ is the noise scaling factor, and $\mathbf{z}$ is Gaussian noise.

Applying a frequency decomposition $\omega = \{\omega_L, \omega_H\}$:
\begin{equation}
    \hat{\mathbf{m}}_{t-1}(\omega) = \big( \hat{\mathbf{m}}_{t-1}(\omega_L), \hat{\mathbf{m}}_{t-1}(\omega_H) \big)
\end{equation}

By the Markov property of the diffusion process, the joint distribution can be decomposed:
\begin{equation}
    p(\hat{\mathbf{m}}_{t-1}(\omega_L), \hat{\mathbf{m}}_{t-1}(\omega_H) \mid \hat{\mathbf{m}}_t(\omega_L), \hat{\mathbf{m}}_t(\omega_H)) = p(\hat{\mathbf{m}}_{t-1}(\omega_L) \mid \hat{\mathbf{m}}_t(\omega_L)) \cdot p(\hat{\mathbf{m}}_{t-1}(\omega_H) \mid \hat{\mathbf{m}}_{t-1}(\omega_L), \hat{\mathbf{m}}_t(\omega_H))
\end{equation}

Due to the dominance of low-frequency components in determining semantic structure, $\hat{\mathbf{m}}_{t-1}(\omega_H)$ strongly depends on the reconstructed $\hat{\mathbf{m}}_{t-1}(\omega_L)$:
\begin{equation}
    p(\hat{\mathbf{m}}_{t-1}(\omega_H) \mid \hat{\mathbf{m}}_{t-1}(\omega_L), \hat{\mathbf{m}}_t(\omega_H)) \approx p(\hat{\mathbf{m}}_{t-1}(\omega_H) \mid \hat{\mathbf{m}}_{t-1}(\omega_L))
\end{equation}

This reflects the fact that high-frequency details align with low-frequency structures, ensuring consistency in motion semantics and spatial coherence.

Furthermore, noise energy $\mathbb{E}[|\hat{\boldsymbol{\epsilon}}_t(\omega_H)|^2]$ in high frequencies $\omega_H$ is significantly higher than that in low frequencies $\omega_L$. This emphasizes that high-frequency components are more corrupted by noise and require low-frequency components for meaningful recovery.

The theorem demonstrates that diffusion-based motion generation inherently follows a hierarchical restoration process, where low-frequency semantic consistency provides the foundation for high-frequency detail recovery. 
%%%%%%%%%%%%%%%%%%%%%%%%%%%%%%%%%%%%%%%%%%%%%%%%%%%%%%%%%%%%%%%%%%%%%%%%%%%%%%%
%%%%%%%%%%%%%%%%%%%%%%%%%%%%%%%%%%%%%%%%%%%%%%%%%%%%%%%%%%%%%%%%%%%%%%%%%%%%%%%

\subsection{Detailed DCT and IDCT Formulas}

\subsubsection{Discrete Cosine Transform (DCT)}
For a signal $\mathbf{v} = \{v[0], v[1], \dots, v[N-1]\}$, the DCT is defined as:
\begin{equation}
    \mathbf{v}_f[k] = \alpha(k) \sum_{n=0}^{N-1} v[n] \cos\left(\frac{\pi (2n + 1)k}{2N}\right), \quad k = 0, 1, \dots, N-1,
\end{equation}

where the normalization factor $\alpha(k)$ is:
\begin{equation}
    \alpha(k) =
\begin{cases}
\sqrt{\frac{1}{N}}, & \text{if } k = 0, \\
\sqrt{\frac{2}{N}}, & \text{if } k > 0.
\end{cases}
\end{equation}

\subsubsection{Inverse Discrete Cosine Transform (IDCT)}
The original signal $\mathbf{v}$ can be recovered from its DCT coefficients $\mathbf{v}_f = \{v_f[0], v_f[1], \dots, v_f[N-1]\}$ using:
\begin{equation}
    v[n] = \sum_{k=0}^{N-1} \alpha(k) v_f[k] \cos\left(\frac{\pi (2n + 1)k}{2N}\right), \quad n = 0, 1, \dots, N-1
\end{equation}

\subsubsection{Low-Frequency Filtering in Batch Processing}
Given a batch $\mathbf{X} \in \mathbb{R}^{B \times N \times D}$, where $B$ is the batch size, $N$ is the time step, and $D$ is the feature dimension, the steps for low-frequency filtering are as follows:

1. Compute the DCT for each feature dimension $d = 1, 2, \dots, D$:
\begin{equation}
    \mathbf{x}_{d,f}[k] = \alpha(k) \sum_{n=0}^{N-1} x_d[n] \cos\left(\frac{\pi (2n + 1)k}{2N}\right), \quad k = 0, 1, \dots, N-1.
\end{equation}

2. Retain only the first $K$ coefficients (low frequencies) and set the rest to zero:
\begin{equation}
    \mathbf{x}_{d,f}[k] =
\begin{cases}
\mathbf{x}_{d,f}[k], & k < K, \\
0, & k \geq K.
\end{cases}
\end{equation}

3. Reconstruct the time-domain signal using IDCT:
\begin{equation}
    \tilde{\mathbf{x}}_d[n] = \sum_{k=0}^{N-1} \alpha(k) \mathbf{x}_{d,f}[k] \cos\left(\frac{\pi (2n + 1)k}{2N}\right), \quad n = 0, 1, \dots, N-1.
\end{equation}

4. Concatenate the filtered signals along the feature dimension:
\begin{equation}
    \mathbf{X}_{\text{filtered}} = \text{Concat}(\tilde{\mathbf{x}}_1, \tilde{\mathbf{x}}_2, \dots, \tilde{\mathbf{x}}_D)
\end{equation}

\section{Evaluation Metrics}
\label{sec:evalmetrics}
\textbf{Frechet Inception Distance (FID)}. FID is used to measure the difference in distribution between generated motions. We have the following formulas to obtain FID:
\begin{align}
    FID &= \| \mu_{gt} - \mu_{pred} \|_2^2 - \text{Tr}(\Sigma_{gt} + \Sigma_{pred} - 2(\Sigma_{gt}\Sigma_{pred})^{1/2})
\end{align}
\\
Here, $\mu$ represents the mean, $\Sigma$ is the covariance matrix, and $\text{Tr}$ denotes the trace of a matrix. The smaller the difference, the less susceptible the model is to perturbation.\\

\textbf{Diversity.}
Diversity can measure the diversity of action sequences. A larger value of the metric indicates better diversity in the model. We randomly sample $S$ pairs of motions, denoted as ${f}_i$ and ${f}_i'$. According to \cite{T2M-GPT}, we set $S$ to be 300.  We can calculate using the following formula:
\begin{align}
    Diversity = \frac{1}{S} \sum_{i=1}^{S} \| {f}_i - {f}_i' \|
\end{align}

\section{Efficiency Analysis}
\label{efficiency}
The proposed method does not impact the inference speed of the model during generation. However, during training, the addition of two extra loss terms, $\mathcal{L}_\text{LF}$ and $\mathcal{L}_\text{S}$, introduces an increased computational cost, resulting in a slower training process. Specifically, as shown in Table~\ref{tab:training_inference_time}, the computational overhead caused by $\mathcal{L}_\text{LF}$ is relatively minor, while $\mathcal{L}_\text{S}$ leads to a more slowdown due to the invocation of an additional model. Because, the efficiency limitations of the DCT transformation algorithm, combined with the computational demands of the motion embedding mechanism, contribute to the reduced training efficiency. Nevertheless, the overall training time increases by $16.7 \%$ for MDM and $12.5 \%$  for StableMoFusion, while the proposed method achieves notable improvements in model performance.

\begin{table}[h]
    \centering
    \begin{tabular}{ccccc}
        \hline
        Time &MDM & Free-MDM & StableMoFusion & Free-StableMoFusion  \\
        \hline
        Training time & 72h & 84h & 96h & 108h \\
        Inference time & 0.045s & 0.045s & 0.036s & 0.036s \\

        \hline
    \end{tabular}
    \caption{Training Time and Inference Time: We conducted our experiments on an NVIDIA 3090 GPU. Training Time refers to the time required for MDM to complete 600,000 steps and StableMoFusion to complete 200,000 steps. Inference Time represents the average time needed by each of the four models to generate 200 samples.}
    \label{tab:training_inference_time}
\end{table}

\section{More Visualization Results}
\label{More visualization}
More visualization results an be found on the \href{https://github.com/Hxxxz0/Free-T2m}{website}.

\section{Motion Data Analysis}
\label{data analysis}

\begin{figure*}[ht]
    \centering
    \includegraphics[width=0.7\linewidth]{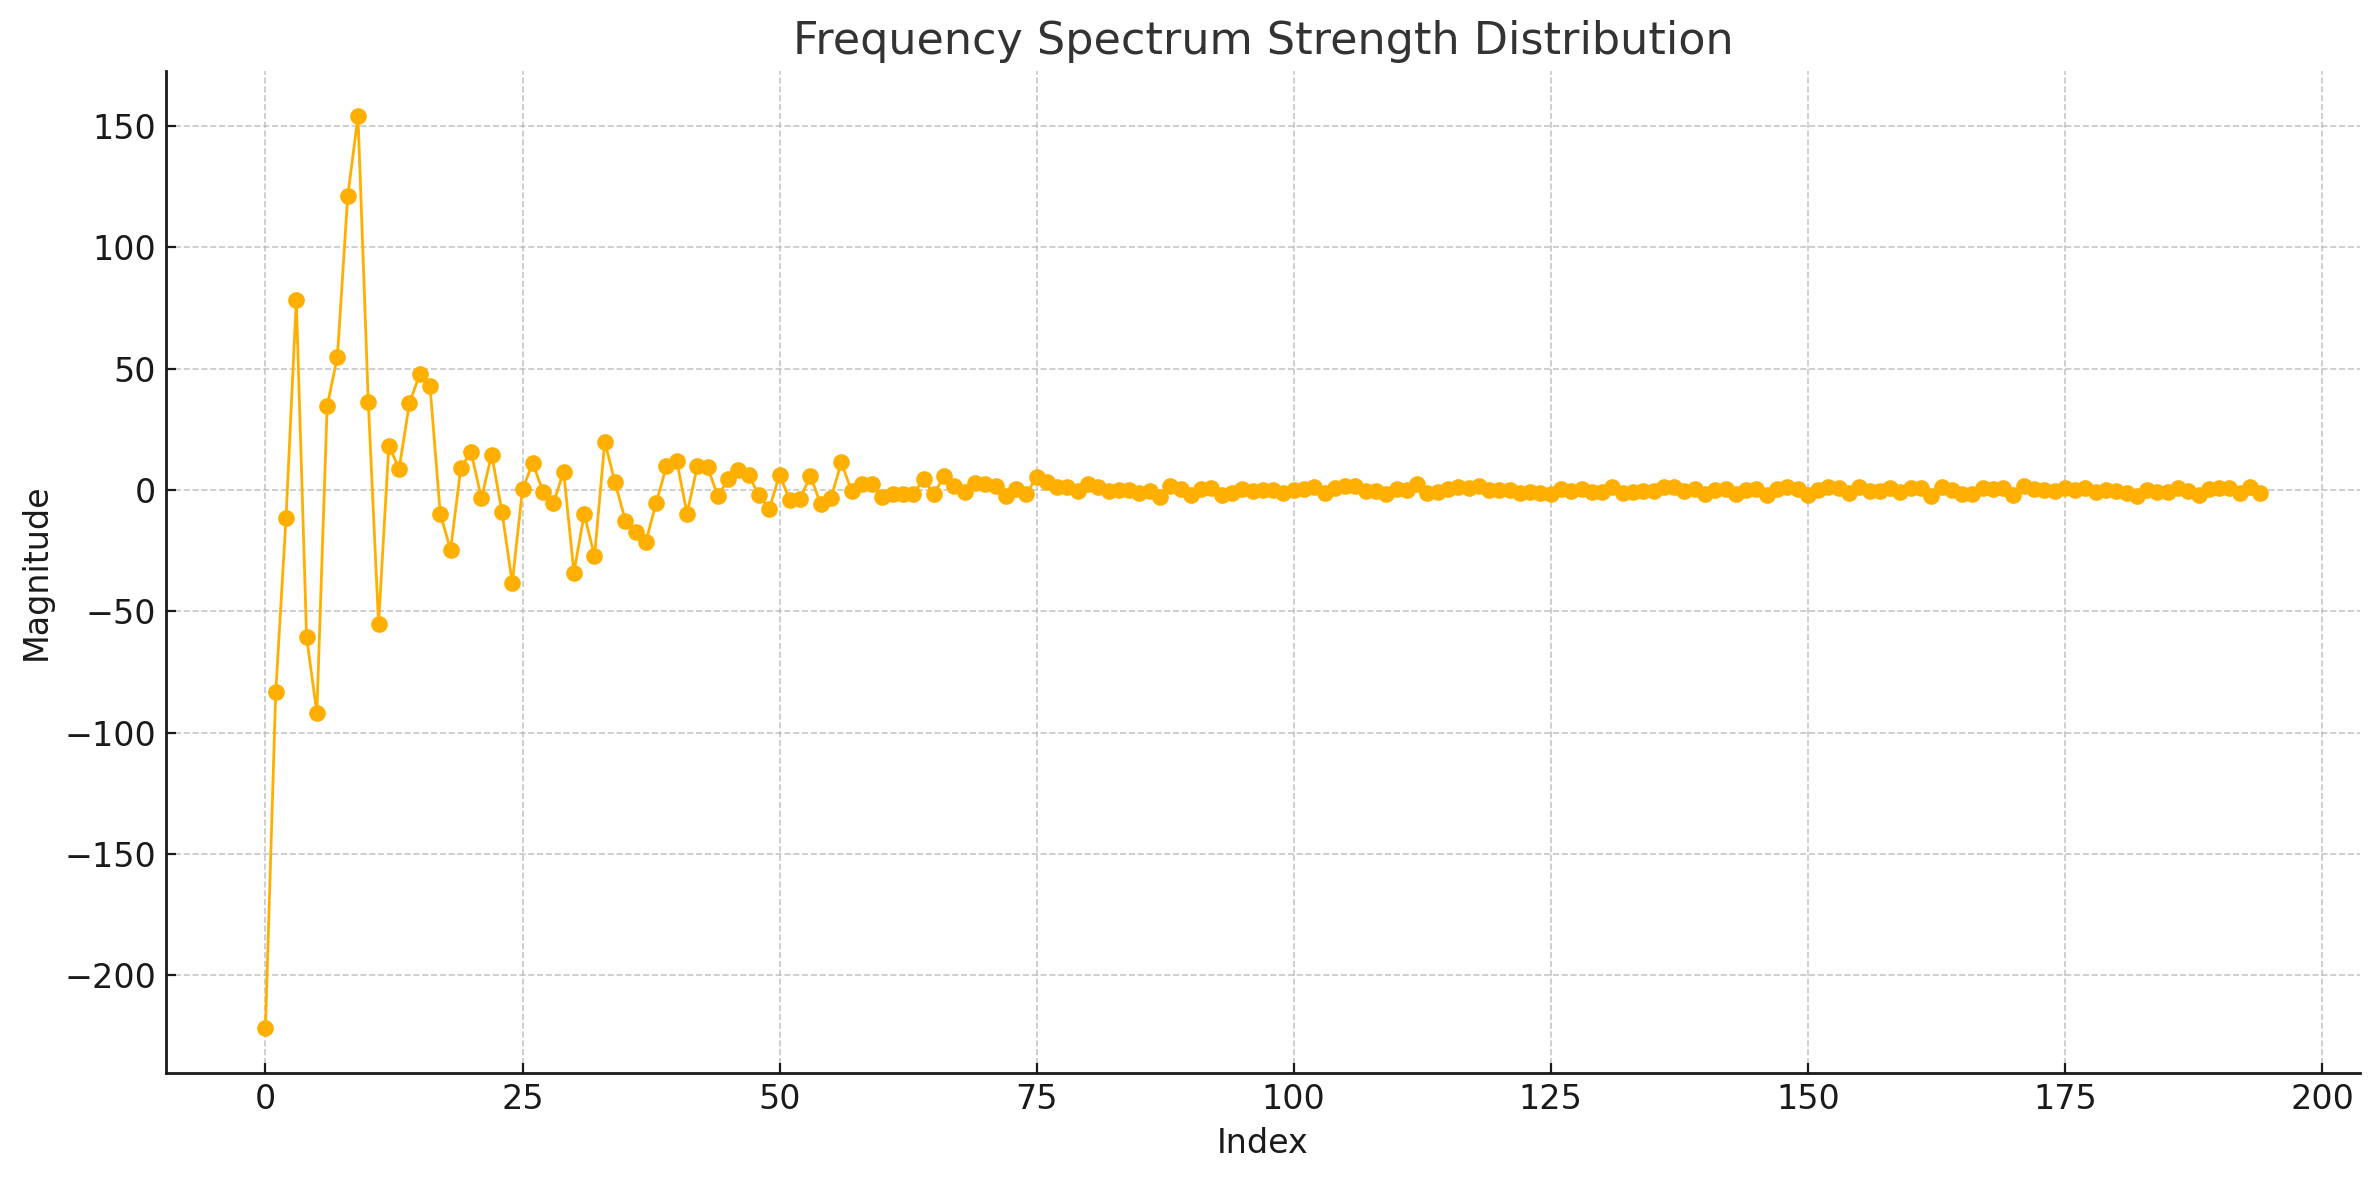}
    \caption{Frequency Spectrum Strength Distribution of Motion Data: This figure illustrates the distribution of motion data after applying the Discrete Cosine Transform (DCT). The results show that motion data is predominantly dominated by low-frequency components, highlighting the importance of focusing on low-frequency information for accurately capturing and generating motion trajectories.}
    \label{fig:frequency}
\end{figure*}

To effectively capture the structural and semantic properties of motion data, we analyze representations commonly used in prior works, focusing on both the \textit{HumanML3D Format} and the \textit{SMPL-based Format}. These representations enable precise motion modeling, providing a robust foundation for text-to-motion generation with enhanced semantic fidelity.

\textbf{HumanML3D Format.} Drawing inspiration from character control techniques, HumanML3D \cite{humanmotion3d} encodes motion as a tuple of diverse features, capturing both spatial and dynamic properties. These include root angular velocity $r^a$ (Y-axis), root linear velocities $r^x, r^z$ (XZ-plane), root height $r^y$, local joint positions $j^P \in \mathbb{R}^{3N_j}$, joint velocities $j^v \in \mathbb{R}^{3N_j}$, joint rotations $j^r \in \mathbb{R}^{6N_j}$, and binary foot-ground contact features $c^f \in \mathbb{R}^4$:
\begin{equation}
x^i = \{r^a, r^x, r^z, r^y, j^P, j^v, j^r, c^f\}.
\end{equation}
This comprehensive definition encapsulates both high-level semantic structures and fine-grained dynamic details, ensuring a holistic motion representation.

\textbf{SMPL-based Format.} The SMPL model \cite{SMPL} emphasizes anatomical accuracy, representing motion through shape parameters $\beta$, pose parameters $\theta \in \mathbb{R}^{3 \times 23 + 3}$, and global translation $r$. Here, $\theta$ encodes rotations for 23 joints and a root joint, while $\beta$ captures individual body shape variations:
\begin{equation}
x^i = \{r, \theta, \beta\}.
\end{equation}
This format is well-suited for modeling biomechanical realism and is widely used in motion generation tasks.

In addition to leveraging these formats, we introduce a novel frequency-domain perspective to analyze motion data. As illustrated in Figure~\ref{fig:frequency}, motion data exhibits a dominance of low-frequency components, which encode broad semantic structures like global trajectories. In contrast, high-frequency components are sparse and primarily capture fine-grained details. This dual-domain analysis lays the groundwork for improving text-to-motion generation by aligning semantic planning with detailed motion refinement.

\section{More Experiments}
\label{more experiments}
\subsection{Loss Coefficient Ablation}

The loss coefficients $\lambda_1$, $\lambda_2$, and $\lambda_3$ correspond to $\mathcal{L}_{\text{simple}}$, $\mathcal{L}_{\text{LF}}$, and $\mathcal{L}_{\text{S}}$, respectively. To determine the optimal values for these coefficients, we conducted experiments with six different parameter combinations, as shown in Table~\ref{tab:parameter_analysis}.

Our results indicate that the proposed method consistently outperforms the baseline metrics (FID: 0.544, R-Top3: 0.611) across most parameter configurations, demonstrating robust performance under various settings.

The best performance was achieved when $\lambda_1$, $\lambda_2$, and $\lambda_3$ were set to 1.0, 1.0, and 0.5, respectively, resulting in an FID of $0.256 ^{\pm 0.045}$ and an R-Top3 of $0.757 ^{\pm 0.005}$. Notably, reducing $\lambda_1$ below 0.5 led to significant model instability, highlighting its critical role in maintaining stable training. For $\lambda_2$, values within the range $0.5-1.0$ provided robust performance, with higher values yielding improved FID scores. Meanwhile, $\lambda_3$ values between $0.25$ and $0.5$ balanced semantic alignment and generation quality, with higher values contributing positively to semantic consistency.

In summary, our experiments suggest that the optimal range for the loss coefficients is $\lambda_1 \in [0.5, 1.0]$, $\lambda_2 \in [0.5, 1.0]$, and $\lambda_3 \in [0.25, 0.5]$. Within these ranges, the model demonstrates strong robustness and achieves superior performance compared to the baseline.
\begin{table}[ht]
\centering
\resizebox{0.5\textwidth}{!}{%
\begin{tabular}{lllll}
\hline
$\lambda_1$ & $\lambda_2$ & $\lambda_3$  & FID$\downarrow$  & R-Top3$\uparrow$ \\ \hline
1.0         & 1.0        & 1.0  & 0.431$^{\pm0.004}$    & 0.736$^{\pm0.021}$ \\
1.0         & 1.0        & 0.5  & 0.256$^{\pm0.045}$          & 0.757$^{\pm0.005}$ \\

0.5         & 1.0        & 1.0  &  0.301$^{\pm0.021}$     & 0.728$^{\pm0.003}$ \\

1.0         & 0.5        & 1.0  &   0.471$^{\pm0.201}$     & 0.733$^{\pm0.014}$ \\

1.0         & 1.0        & 0.25  & 0.398$^{\pm0.121}$    & 0.755$^{\pm0.011}$ \\
1.0         & 0.25        & 1.0  & 0.592$^{\pm0.001}$    & 0.701$^{\pm0.022}$ \\
0.25         & 1.0        & 1.0  & 1.134$^{\pm0.117}$    & 0.607$^{\pm0.074}$ \\

\hline
\end{tabular}%
}
\caption{Parameter analysis. $\pm$ indicates a 95\% confidence interval. 
R-Top3 represents R-Precision Top3. The table displays the results of three different parameters for loss.}
\label{tab:parameter_analysis}
\end{table}

\subsection{Fine-Tuning vs. Training}
% \begin{table*}[htbp]
% \centering
% \resizebox{0.8\textwidth}{!}{%
% \begin{tabular}{lccccc}
% \hline
% \textbf{Method} & \textbf{FID $\downarrow$} & \multicolumn{3}{c}{\textbf{R-Precision $\uparrow$}} & \textbf{Diversity $\rightarrow$} \\ \cline{3-5}
%  &  & \textbf{top1} & \textbf{top2} & \textbf{top3} \\ \hline

% \(\mathcal{L_\text{LF}} + \mathcal{L}_\text{S}\)    
%                               & $\mathbf{0.261^{\pm0.043}}$ & $\mathbf{0.466^{\pm0.008}}$ & $\mathbf{0.657^{\pm0.007}}$ & $\mathbf{0.757^{\pm0.005}}$ & $9.666^{\pm0.078}$ \\ 

% \(\mathcal{L}_\text{LF}\) only        & $0.444^{\pm0.003}$ & $0.456^{\pm0.004}$ & $0.652^{\pm0.001}$ & $0.759^{\pm0.001}$ & $9.637^{\pm0.005}$ \\ 

% \(\mathcal{L}_\text{S}\) only        & $0.731^{\pm0.066}$ & $0.4305^{\pm0.007}$ & $0.619^{\pm0.006}$ & $0.722^{\pm0.006}$ & $\mathbf{9.464^{\pm0.076}}$ \\ \hline
% \end{tabular}%
% }
% \caption{Ablation experiment results of MDM$_{50steps}$ for \(\mathcal{L}_\text{LF}\) and \(\mathcal{L}_\text{S}\) on the HumanML3D test set. Bold indicates the best result.}
% \label{table:ablation_results}
% \end{table*}

\begin{table}[t]
\centering
\resizebox{0.9\linewidth}{!}{%
\begin{tabular}{lcccc}
\hline
\textbf{Method} & \textbf{FID $\downarrow$} & \multicolumn{3}{c}{\textbf{R-Precision $\uparrow$}}  \\ \cline{3-5}
 &  & \textbf{top1} & \textbf{top2} & \textbf{top3} \\ \hline
StableMoFusion (Baseline)& $0.189^{\pm0.003}$ & $0.499^{\pm0.004}$ & $0.680^{\pm0.006}$ & $0.779^{\pm0.007}$  \\ 
Free-StableMoFusion (Training)  & $\mathbf{0.051^{\pm0.002}}$ & $0.520^{\pm0.013}$ &$0.707^{\pm0.003}$ & $0.803^{\pm0.006}$ \\
Free-StableMoFusion (Fine-tuning)  
                              & $0.091^{\pm0.011}$ & $\mathbf{0.535^{\pm0.004}}$ & $\mathbf{0.728^{\pm0.041}}$ & $\mathbf{0.819^{\pm0.002}}$    \\ \hline
\end{tabular}%
}
\caption{Different training approaches for StableMoFusion: Fine-tuning the existing model using Free-T2M is more efficient and effective.}
\label{table:fine-tuning}

\end{table}

We investigated two training strategies for our method: training from scratch and fine-tuning on a pre-trained model using our proposed approach. Using StableMoFusion as the baseline, we conducted experiments with both methods. For training from scratch, we set the total training steps to 200,000, while fine-tuning was carried out for 100,000 steps. The results, as presented in Table \ref{table:fine-tuning}, show that both approaches outperform the baseline, with each offering unique advantages.

Specifically, training from scratch achieved superior performance in FID, while fine-tuning excelled in R-Precision, achieving state-of-the-art results. These findings demonstrate the versatility of our method: it can serve as an effective strategy to enhance performance during the training process for T2M tasks or as a powerful tool to further refine and improve the accuracy of pre-trained models. Furthermore, the exceptional performance of fine-tuning underscores the efficiency of our approach, offering a resource-conscious yet highly effective alternative for performance optimization.

\subsection{R-Precision Under Different Sample Sizes.}
\label{R-Precision under different sample sizes}
In most previous works, the sampled texts for R-Precision evaluation consist of 32 candidates (1 ground truth and 31 randomly sampled test texts). The results for Top-1, Top-2, and Top-3 are obtained through ranking and repeated calculations. In this paper, to provide a more rigorous comparison of this metric across different models, we experimented with a broader range of sampled text quantities, using StableMoFusion as the baseline. The results, shown in Table \ref{table:sample}, indicate that our method consistently outperforms the baseline across all sampling sizes (8, 16, 32, and 64). This demonstrates that our approach achieves significantly better semantic alignment, further validating its effectiveness.
% Please add the following required packages to your document preamble:
% \usepackage{multirow}
% \usepackage{graphicx}
\begin{table}[ht]
\centering
\resizebox{0.5\columnwidth}{!}{%
\begin{tabular}{lclll}
\hline
Method                   & \multicolumn{1}{l}{Num} & Top-1 & Top-2 & Top-3 \\ \hline
Real                     & \multirow{3}{*}{8}      &0.771       & 0.912      &  0.962     \\
Free-StableMoFusion      &                         & \textbf{0.775}      & \textbf{0.923}      & \textbf{0.969}      \\
StableMoFusion(baseline) &                         &   0.753    & 0.909      & 0.962      \\ \hline
Real                     & \multirow{3}{*}{16}     &  0.646     &  0.820     & 0.900      \\
Free-StableMoFusion      &                         &  \textbf{0.657}     & \textbf{0.841}      & \textbf{0.913}      \\
StableMoFusion(baseline) &                         & 0.634      & 0.816      & 0.892      \\ \hline
Real                     & \multirow{3}{*}{32}     &0.511       &  0.703     &  0.797     \\
Free-StableMoFusion      &                         & \textbf{0.520}      & \textbf{0.707}      & \textbf{0.803}      \\
StableMoFusion(baseline) &                         & 0.499      & 0.681      &0.779       \\ \hline
Real                     & \multirow{3}{*}{64}     &   0.374      &  0.560     & 0.672      \\
Free-StableMoFusion      &                         & \textbf{0.394}      &  \textbf{0.566}     &   \textbf{0.678}    \\
StableMoFusion(baseline) &                         &  0.378      &  0.550     & 0.647      \\ \hline

\end{tabular}%

}

\caption{R-Precision Results with Different Numbers of Sampled Texts. Our method achieves higher accuracy than the baseline across all sampling sizes, further demonstrating its ability to improve semantic consistency in generated results.}
\label{table:sample}
\end{table}

% Real                     & \multirow{3}{*}{128}    &       &       &       \\
% Free-StableMoFusion      &                         &       &       &       \\
% StableMoFusion(baseline) &                         &       &       &       \\ \hline

\subsection{Mask Strategy Ablation.}
An important finding in our work is that the denoising process of diffusion models can be divided into two distinct stages. During the semantic planning stage, we introduce a low-frequency consistency loss, while in the fine-grained improving stage, we propose a semantic consistency loss. Using a mask mechanism, we apply the low-frequency consistency loss only in the early stages and the semantic consistency loss in the later stages. This approach aligns with intuitive reasoning: during the early stages, actions are dominated by disordered noise, making it difficult to capture semantic properties, so applying semantic consistency at this point is ineffective. Conversely, as the denoising process advances into the later stages, low-frequency semantic generation is largely completed. Persistently emphasizing low-frequency generation at this stage would hinder the optimization of high-frequency details. Our experimental results support this rationale (see Table \ref{table:mask_ablation}). Across two different models, applying the mask strategy consistently improves both accuracy and semantic alignment compared to not using the mask strategy.
\begin{table*}[htbp]
\centering
\resizebox{\textwidth}{!}{%
\begin{tabular}{lccccc}
\hline
\textbf{Method} & \textbf{FID $\downarrow$} & \multicolumn{3}{c}{\textbf{R-Precision $\uparrow$}} & \textbf{Diversity $\rightarrow$} \\ \cline{3-5}
 &  & \textbf{top1} & \textbf{top2} & \textbf{top3} \\ \hline

NO-Mask Free-MDM    
& $0.310^{\pm0.040}$ 
& $0.452^{\pm0.007}$ 
& $0.648^{\pm0.006}$ 
& $0.755^{\pm0.005}$ 
& $9.824^{\pm0.101}$ \\ 

Mask Free-MDM   
&  $\mathbf{0.261^{\pm0.043}}$
& $\mathbf{0.466^{\pm0.008}}$ 
    & $\mathbf{0.657^{\pm0.007}}$ 
& $\mathbf{0.757^{\pm0.005}}$
&  $\mathbf{9.666^{\pm0.080}}$ \\

No-Mask Free-StableMoFusion   
& $0.103^{\pm0.032}$ & $0.491^{\pm0.006}$ & $0.673^{\pm0.012}$ & $0.769^{\pm0.009}$ & $9.110^{\pm0.088}$
 \\ 
Mask Free-StableMoFusion   
& $\mathbf{0.051^{\pm0.002}}$ & $\mathbf{0.520^{\pm0.003}}$ & $\mathbf{0.707^{\pm0.003}}$ & $\mathbf{0.803^{\pm0.006}}$ & $\mathbf{9.480^{\pm0.005}}$\\
\hline
\end{tabular}%
}
\caption{Mask strategy ablation. $\pm$ indicates a 95\% confidence interval. Bold text highlights superior results. Across different baselines, the mask strategy can improve model performance, demonstrating the necessity of applying two distinct consistencies during the denoising stages.}
\label{table:mask_ablation}
\end{table*}

\section{Details of Human Evaluation}
\label{app:human_eval}
We sampled 100 test texts and manually evaluated the results generated by Free-MDM, MDM, Free-StableMoFusion, and StableMoFusion. Below is the Google Form format we used for the evaluation:
\definecolor{myTealLight}{rgb}{0.2, 0.8, 0.8} 

\begin{tcolorbox}[colback=gray!20,arc=2mm,boxrule=0.5mm,colframe=red!70!black,title=Details of Human Evaluation]
\textbf{\textcolor{red}{[Question1]: }} Do you think the motion in GIF 1 is correct?  \par
% \vspace{2mm}
\begin{enumerate}
    \item Yes
    \item No
    
\end{enumerate}

% \vspace{5mm}
\textbf{\textcolor{red}{[Question2]: }} Do you think the motion in GIF 2 is correct?\par
% \vspace{2mm}
\begin{enumerate}
     \item Yes
    \item No
\end{enumerate}

% \vspace{5mm}
\textbf{\textcolor{red}{[Question3]: }} Based on factors such as motion naturalness, semantic alignment, accuracy, and completeness, which motion result do you prefer? (Please consider these criteria holistically when making your choice.) \par
% \vspace{2mm}
\begin{enumerate}
    \item GIF 1
    \item GIF 1
\end{enumerate}
\end{tcolorbox}
